# Supplementary material for: Regularized Optimal Transport Layers for Generalized Global Pooling Operations
Source: arXiv:2212.06339 source file (2022-12-13)
Supplement: Supplementary file 1 [file appendix.tex]

\appendices
\section{The Delayed Proofs}

\section{More Detailed Derivations}
\textit{The derivation of~\eqref{eq:dual3}.}
According to~\cite{pham2020unbalanced}, we can first formulate the Fenchel's dual form of~\eqref{eq:euot_prob} as follows:
\begin{eqnarray}\label{eq:dual1}
\begin{aligned}
    \sideset{}{_{\bm{a}\in\mathbb{R}^D,\bm{b}\in\mathbb{R}^N}}\min &(\alpha_1+\tau)\sideset{}{_{d,n=1}^{D,N}}\sum \exp\Bigl( \frac{a_d+b_n + c^{(t)}_{dn}}{\alpha_1 + \tau} \Bigr)\\
    &+F^*(-\bm{a}) + G^*(-\bm{b}),
\end{aligned}
\end{eqnarray}
where $\bm{a}$ and $\bm{b}$ are dual variables, and
\begin{eqnarray}\label{eq:dual2}
\begin{aligned}
    F^*(\bm{a})&=\sideset{}{_{\bm{z}\in\mathbb{R}^D}}\max\bm{z}^T\bm{a}-\alpha_2 \text{KL}(\bm{z} | \bm{p}_0)\\
    &=\alpha_2\Bigl\langle\exp\Bigl(\frac{1}{\alpha_2}\bm{a}\Bigr) - \bm{1}_D, \bm{p}_0\Bigr\rangle.\\
    G^*(\bm{b})&=\sideset{}{_{\bm{z}\in\mathbb{R}^N}}\max\bm{z}^T\bm{b}-\alpha_3 \text{KL}(\bm{z} | \bm{q}_0)\\
    &=\alpha_3\Bigl\langle\exp\Bigl(\frac{1}{\alpha_3}\bm{b}\Bigr) - \bm{1}_N, \bm{q}_0\Bigr\rangle.
\end{aligned}
\end{eqnarray}
Plugging~\eqref{eq:dual2} into~\eqref{eq:dual1}, we obtain~\eqref{eq:dual3}.

\textit{The derivations of~\eqref{eq:deriveP} and~\eqref{eq:deriveS}.}
Denote the objective function in~\eqref{eq:updateP} as $L_{\bm{P}}$. 
The detailed derivation of~\eqref{eq:deriveP} is shown as follows:
\begin{eqnarray}
\begin{aligned}
&\frac{\partial L_{\bm{P}}}{\partial\bm{P}}=\bm{0}\\ 
&\Rightarrow\bm{P}=\exp\Bigl(\frac{\bm{X}+\alpha_0\bm{\Sigma}_1\bm{S}^{(t)}\bm{\Sigma}_2^T-\bm{Z}^{(t)}}{\rho}+\log\bm{S}^{(t)}\Bigr)\\
&\xRightarrow{\text{Project to $\Pi(\bm{\mu}^{(t)},\cdot)$}}\bm{P}^{(t+1)}=\\ 
&\text{diag}(\bm{\mu}^{(t)})\sigma_{\text{row}}\Bigl(\underbrace{\frac{\bm{X}+\alpha_0\bm{\Sigma}_1\bm{S}^{(t)}\bm{\Sigma}_2^T-\bm{Z}^{(t)}}{\rho}+\log\bm{S}^{(t)}}_{\text{Denoted as~}\bm{Y}}\Bigr)\\
&\xRightarrow{\text{Logarithmic Update}}\\
&\log\bm{P}^{(t+1)}=(\log\bm{\mu}^{(t)}-\text{LogSumExp}_{\text{row}}(\bm{Y}))\bm{1}_N^T+\bm{Y}.
\end{aligned}
\end{eqnarray}
where $\sigma_{\text{row}}$ is a row-wise softmax operation. 
% When applying the quadratic regularizer, we just need to replace the $\bm{Y}$ with
% \begin{eqnarray*}
%     \frac{\bm{X}-\alpha_0\bm{\Sigma}_1\bm{S}^{(t)}\bm{\Sigma}_2^T-\alpha_1\bm{S}^{(t)}-\bm{Z}^{(t)}}{\rho} + \log\bm{S}^{(t)}.
% \end{eqnarray*}
Similarly, denote the objective function in~\eqref{eq:updateS} as $L_{\bm{S}}$. 
The detailed derivation of~\eqref{eq:deriveS} is shown below:
\begin{eqnarray}
\begin{aligned}
&\frac{\partial L_{\bm{S}}}{\partial\bm{S}}=\bm{0}\\
&\Rightarrow \bm{S}=\exp\Bigl(\frac{\bm{Z}^{(t)}+\alpha_0\bm{\Sigma}_1^T\bm{P}^{(t+1)}\bm{\Sigma}_2 +\rho\log\bm{P}^{(t+1)}}{\alpha_1+\rho}\Bigr)\\
&\xRightarrow{\text{Project to $\Pi(\cdot, \bm{\eta}^{(t)})$}}\bm{S}^{(t+1)}=\\ &\sigma_{\text{col}}\Bigl(\underbrace{\frac{\bm{Z}^{(t)}+\alpha_0\bm{\Sigma}_1^T\bm{P}^{(t+1)}\bm{\Sigma}_2+\rho\log\bm{P}^{(t+1)}}{\alpha_1+\rho}}_{\text{Denoted as~}\bm{Y}}\Bigr)\text{diag}(\bm{\eta}^{(t)})\\
&\xRightarrow{\text{Logarithmic Update}}\\
&\log\bm{S}^{(t+1)}=\bm{1}_D(\log\bm{\eta}^{(t)}-\text{LogSumExp}_{\text{col}}(\bm{Y}))^T +\bm{Y},
\end{aligned}
\end{eqnarray}
where $\sigma_{\text{col}}$ is a column-wise softmax operation.
% Similarly, when applying the quadratic regularizer, we just need to replace the $\bm{Y}$ with
% \begin{eqnarray*}
%     \frac{\alpha_0\bm{\Sigma}_1^T\bm{P}^{(t+1)}\bm{\Sigma}_2-\alpha_1 \bm{P}^{(t+1)}+\bm{Z}^{(t)}}{\rho} + \log \bm{P}^{(t+1)}.
% \end{eqnarray*}
